# Supplementary material for: Deterministic Integration of hBN Single-Photon Emitters on SiN Waveguides via Femtosecond Laser Processing
Source: arXiv:2504.19477 ancillary file (2025-04-28)
Supplement: Supplementary file 1 [file hBN_SPE_waveguide_SI.pdf]

# Supporting Information for
# "Deterministic Integration of hBN Single-Photon Emitters on SiN Waveguides via Femtosecond Laser Processing"

Daiki Yamashita,[1,*] Masaki Yumoto,[2] Aiko Narazaki,[2] and Makoto Okano[3]

[1] *Optical Computing Research Team, Photonics-Electronics Integration Research Center, National Institute of Advanced Industrial Science and Technology (AIST), Ibaraki 305-8568, Japan*

[2] *Laser Processing Frontier Research Group, Core Manufacturing Technology Research Institute, National Institute of Advanced Industrial Science and Technology (AIST), Ibaraki 305-8568, Japan*

[3] *Photo-Electronics Integration Research Team, Photonics-Electronics Integration Research Center, National Institute of Advanced Industrial Science and Technology (AIST), Ibaraki 305-8568, Japan*

[*] Corresponding Author: daiki.yamashita@aist.go.jp

## S1. Deterministic hBN defect creation using femtosecond laser processing

To enable precise laser processing, we employed a single femtosecond laser pulse. The use of a single ultrashort laser pulse reduces heat generation and avoids collateral damage typically associated with high-repetition-rate laser processing [S1, S2]. Figure S1 shows the constructed femtosecond laser system with a wavelength of 520 nm and a pulse width of 344 fs (Spectra Physics: Spirit). The pulse energy was finely tuned using a half-wave plate and a polarized beam splitter, and monitored with an energy meter. The laser was tightly focused onto the sample using an objective lens with a numerical aperture (NA) of 0.95, enabling sub-micron spatial resolution for precise alignment. Laser processing was performed while monitoring the sample with a camera, and the pulse energy was adjusted to identify the appropriate processing threshold. Using this laser system, we fabricated nanoscale optical defects suitable for single-photon emission.

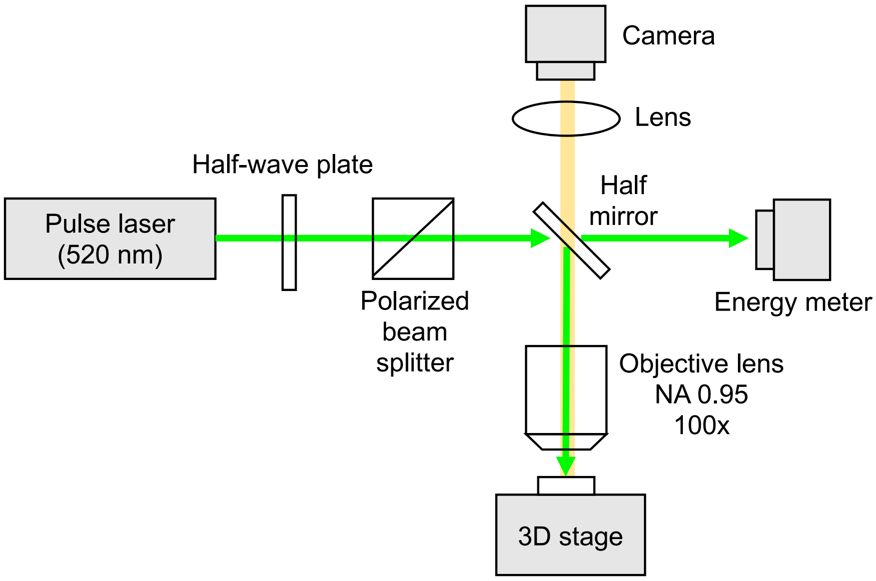


Figure S1. Schematic of the femtosecond laser processing system used for deterministic defect creation.

## S2. Optical characterization and photon correlation measurements

Optical measurements were conducted using a homebuilt micro-photoluminescence (PL) spectroscopy setup, schematically shown in Fig. S2. A continuous-wave (CW) 488 nm laser was used for excitation. The beam was reflected by a dichroic mirror (cutoff wavelength: 500 nm) and focused onto the sample using a 0.9 NA objective lens. Excitation intensity was controlled using a neutral density filter, and polarization was adjusted via a half-wave plate.

The sample was mounted on a 3-axis feedback-controlled translation stage. PL intensity maps were acquired by scanning the stage. To allow independent scanning of the excitation position while keeping the collection spot fixed, a 4f beam-steering configuration using two pairs of relay lenses was implemented. Emission from the sample was transmitted through the dichroic mirror and filtered with a 500 nm long-pass filter. The beam was then directed via a flipper mirror into either a multi-mode fiber (MMF) or single-mode fiber (SMF) for spectroscopic or single-photon counting measurements, respectively. The MMF-coupled light was detected by a spectrometer (YIXIST: YSM-8103-04-01) for PL spectrum acquisition. Light collected via the SMF was split by a 50:50 fiber beam splitter and directed to two single-photon avalanche diodes (SPADs, MPD: PDM FC), with photon events recorded using a time-correlated single-photon counting (TCSPC) module (Swabian Instruments: Time Tagger Ultra). Second-order photon correlation curves were obtained using this Hanbury Brown–Twiss (HBT) setup. All measurements were conducted under ambient conditions at room temperature.

To estimate the photon collection efficiency of the system, we measured the transmission and coupling efficiencies of each optical element using a calibrated power meter. The transmission efficiency of the objective lens was 63.5%, and coupling efficiency into the SMF was 13.5%. The fiber beam splitter had a 50:50 split ratio, the dichroic mirror had a transmission of 95%, and the SPAD quantum efficiency was 43%. Based on these values, the total photon collection efficiency of the optical system was estimated to be 1.75%.

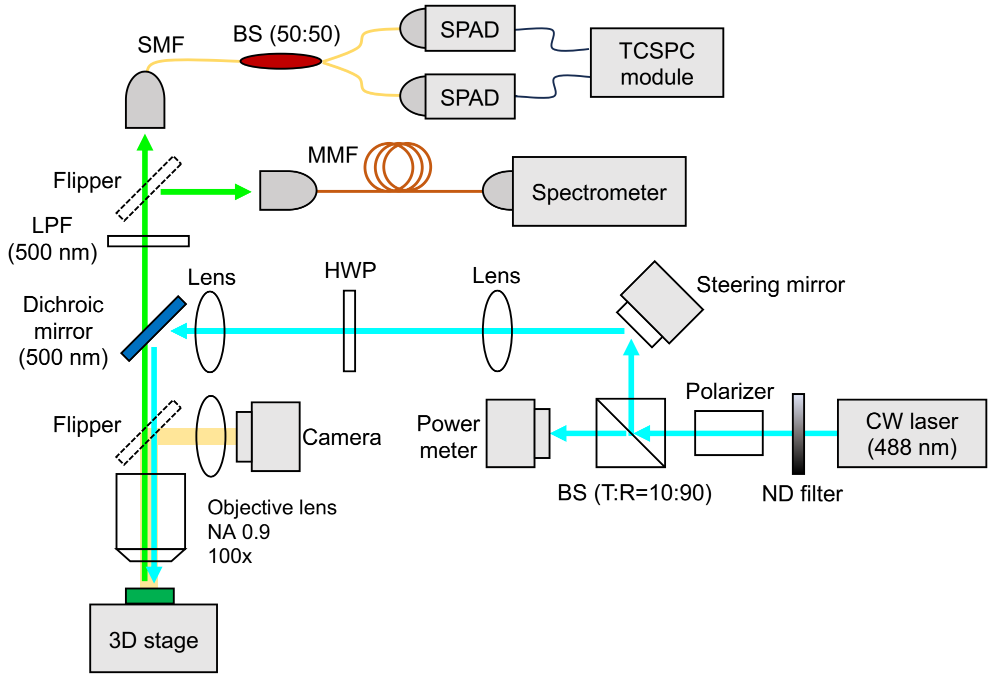


Fig. S2. Schematic of custom-build optical characterization system. Abbreviations: BS – beam splitter; HWP – half-wave plate; LPF – long-pass filter; SMF – single-mode fiber; MMF – multi-mode fiber; SPAD – single-photon avalanche diode; TCSPC – time-correlated single-photon counting.

**S3. Excitation power dependence of second-order correlation curves for the S3 defect.**

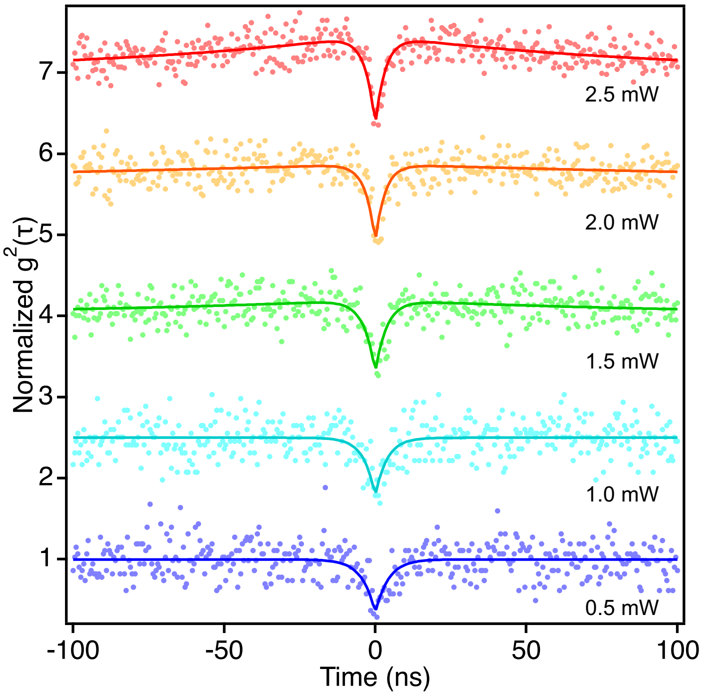


Fig. S3. Excitation power dependence of $g^{(2)}(\tau)$ curves for the S3 defect. Vertical offsets are applied to each curve for clarity. The plots cover excitation powers ranging from 0.5 mW to 2.5 mW. For excitation powers of 0.5 mW and 1.0 mW, the data were fitted using the equation $g^{(2)}(\tau) = 1 - a\ \exp(-|t|/\tau_1)$. For higher powers of 1.5 mW, 2.0 mW, and 2.5 mW, the fitting used the equation $g^{(2)}(\tau) = 1 - a\ \exp(-|t|/\tau_1) - b\ \exp(-|t|/\tau_2)$. At higher excitation powers, the curves exhibit behavior typical of three-level single-photon emitters with a long-lived metastable state [S3].

## S4. Atomic force microscope images of defect patterns

Figures S4 (a-d) show atomic force microscope (AFM) images for S1-S4 defects. Among the defects, the S2 and S3 defect displays a clear bubble-like morphology. In contrast, no distinct surface features are observed for the S1 and S4 defects. Although the same pulse energy was used in all cases, variations in morphology are attributed to substrate and hBN flake inhomogeneities and potential misalignment in the laser writing process [S2, S4, S5].

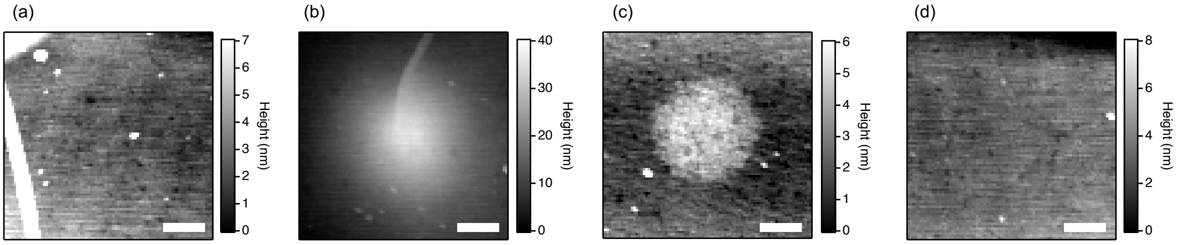


**Fig. S4.** (a–d) AFM images of laser-written defects (S1–S4) shown in Fig. 1(c). All defects were processed with a single pulse at 16.9 nJ pulse energy. The scale bars represent 200 nm, and the thickness of the hBN flake was approximately 30 nm.

## References

S1. S. Eaton, H. Zhang, P. Herman, F. Yoshino, L. Shah, J. Bovatsek, and A. Arai, "Heat accumulation effects in femtosecond laser-written waveguides with variable repetition rate," Opt. Express 13, 4708 (2005).

S2. L. Gan, D. Zhang, R. Zhang, Q. Zhang, H. Sun, Y. Li, and C.-Z. Ning, Large-scale, high-yield laser fabrication of bright and pure single-photon emitters at room temperature in hexagonal boron nitride, ACS Nano 16, 14254 (2022).

S3. Neu, E., Agio, M. & Becher, C. Photophysics of single silicon vacancy centers in diamond: implications for single photon emission. Opt. Express 20, 19956-19971 (2012).

S4. S. Hou, M. D. Birowosuto, S. Umar, M. A. Anicet, R. Y. Tay, P. Coquet, B. K. Tay, H. Wang, and E. H. T. Teo, Localized emission from laser-irradiated defects in 2d hexagonal boron nitride, 2D Materials 5, 015010 (2017).

S5. X.-J. Wang, H.-H. Fang, Z.-Z. Li, D. Wang, and H.-B. Sun, Laser manufacturing of spatial resolution approaching quantum limit, Light: Sci. Appl. 13, 6 (2024).
